# Supplementary material for: Generative Modeling of Discrete Joint Distributions by E-Geodesic Flow Matching on Assignment Manifolds
Source: arXiv:2402.07846 source file (2024-02-12)
Supplement: Supplementary file 1 [file Appendix_B.tex]

% !TEX root =  ../AF_Generative-Discrete_uai2024.tex

\begin{figure}[ht]
	\centering
	\begin{subfigure}{1.\textwidth}
		\includegraphics[width=\textwidth]{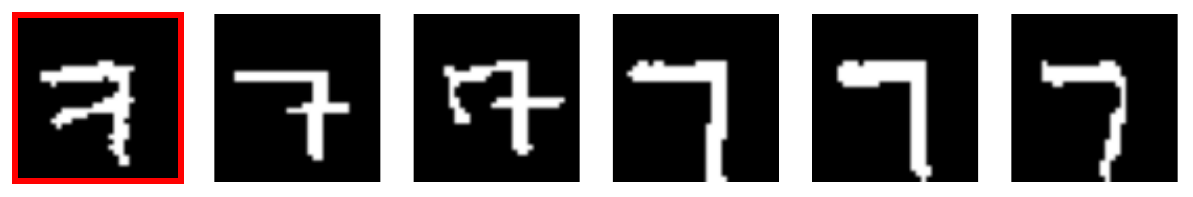}
		%\caption{SubFig 1}
	\end{subfigure}
%%%%%%%%%%%%%%
	\begin{subfigure}{1.\textwidth}
		\includegraphics[width=\textwidth]{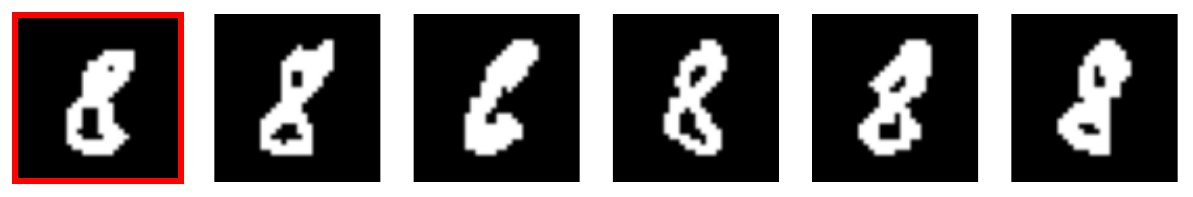}
	\end{subfigure}
%%%%%%%%%%%%%%
	\begin{subfigure}{1.\textwidth}
		\includegraphics[width=\textwidth]{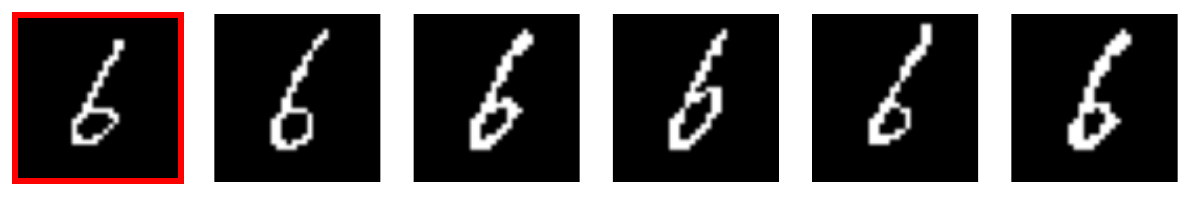}
	\end{subfigure}
%%%%%%%%%%%%%%
	\begin{subfigure}{1.\textwidth}
		\includegraphics[width=\textwidth]{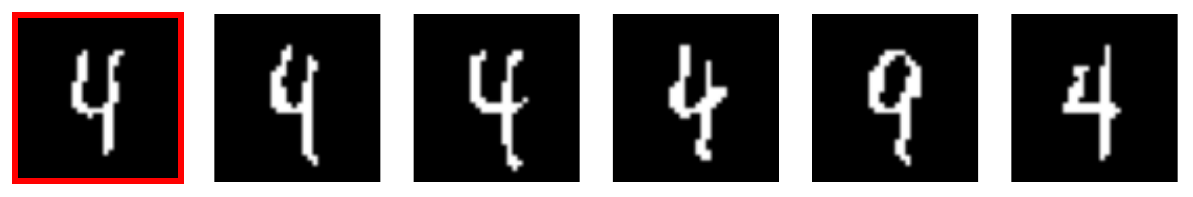}
	\end{subfigure}
	\caption{Illustration of handwritten digit samples trained from the MNIST dataset. The leftmost column, highlighted with a red frame, displays random samples generated by our model through integration Eq. \eqref{eq:def-AF} with random initializations. The remaining plots depict the five closest training samples to our model's instance based on pixel-wise distances. This example serves to demonstrate that our model does not simply memorize the training data.} \label{fig:MNIST_similarity}
\end{figure}

\begin{figure}[h]
	\centering
	\begin{subfigure}{1.\textwidth}
		\includegraphics[width=\textwidth]{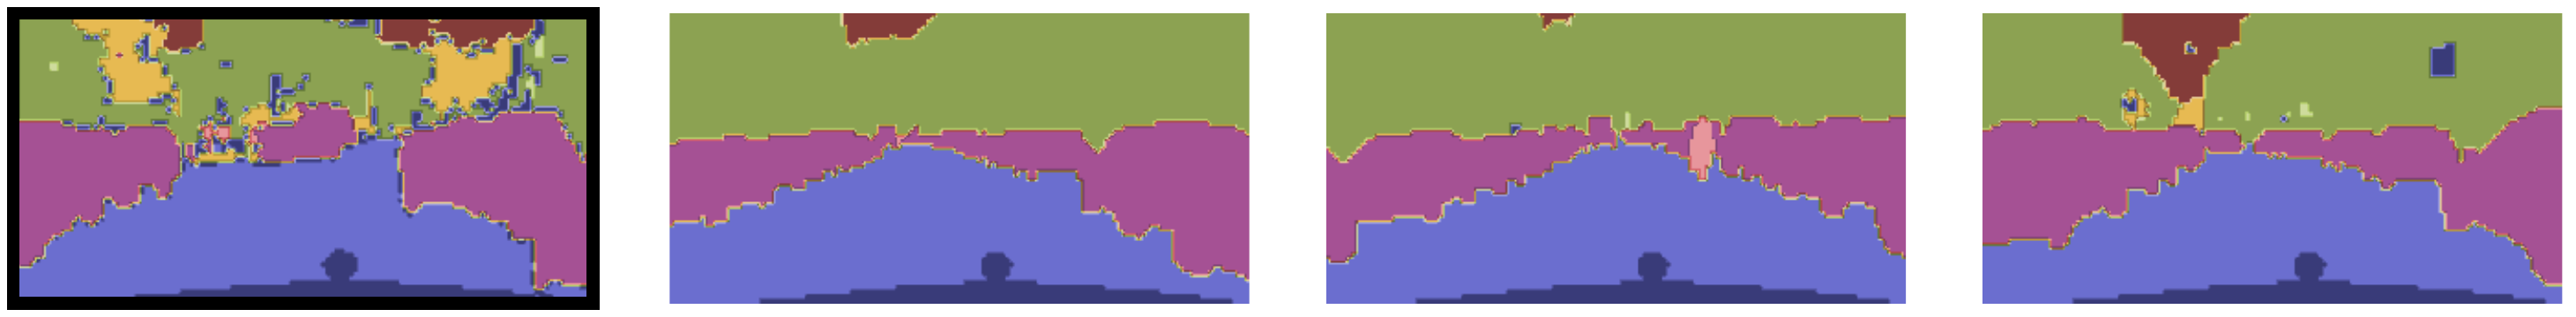}
		%\caption{SubFig 1}
	\end{subfigure}
%%%%%%%%%%%%%%
	\begin{subfigure}{1.\textwidth}
		\includegraphics[width=\textwidth]{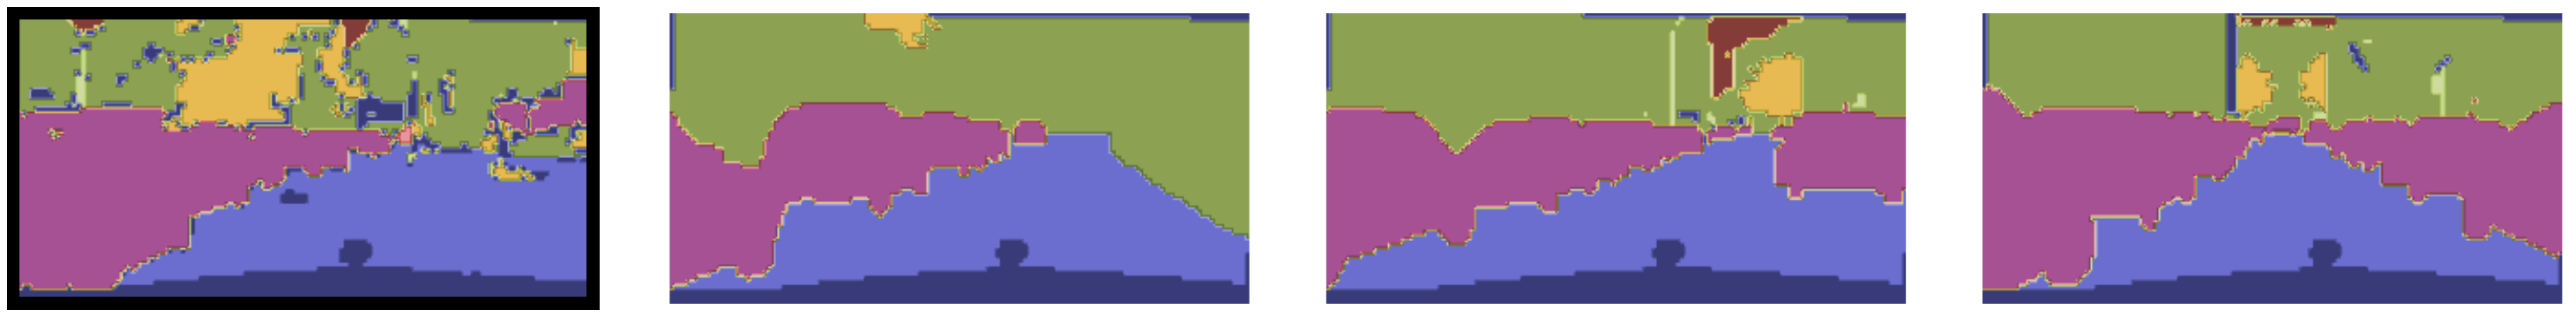}
	\end{subfigure}
%%%%%%%%%%%%%%
	\begin{subfigure}{1.\textwidth}
		\includegraphics[width=\textwidth]{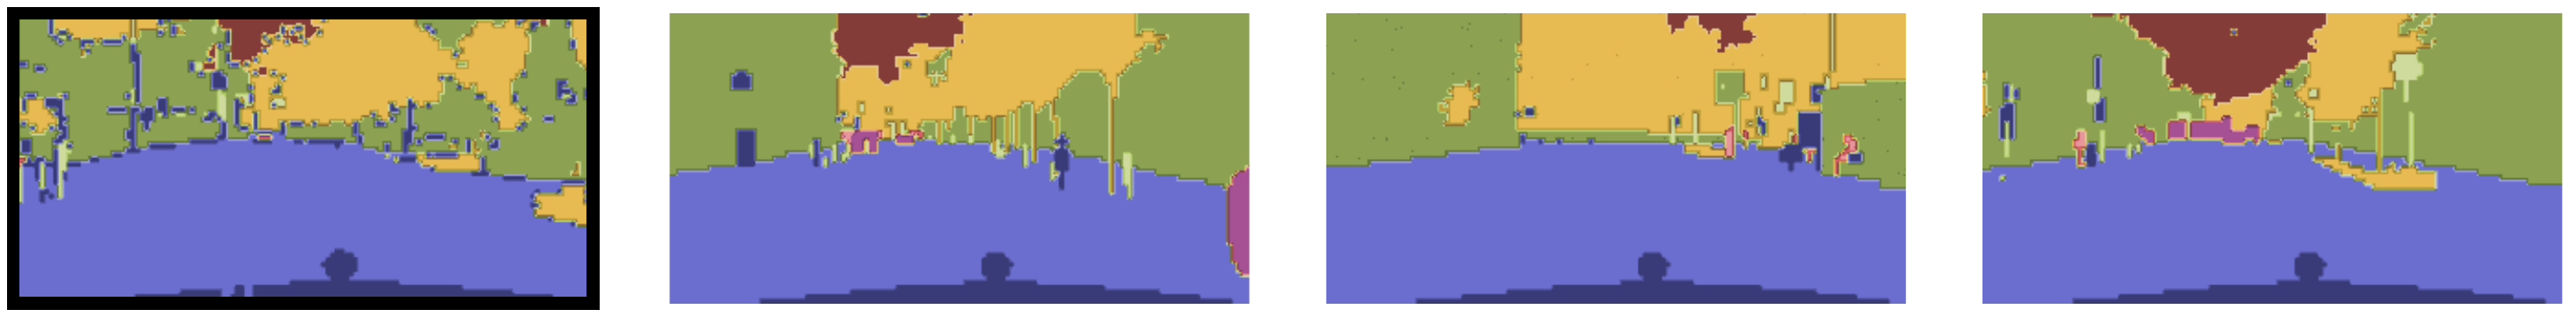}
	\end{subfigure}
%%%%%%%%%%%%%%
	\begin{subfigure}{1.\textwidth}
		\includegraphics[width=\textwidth]{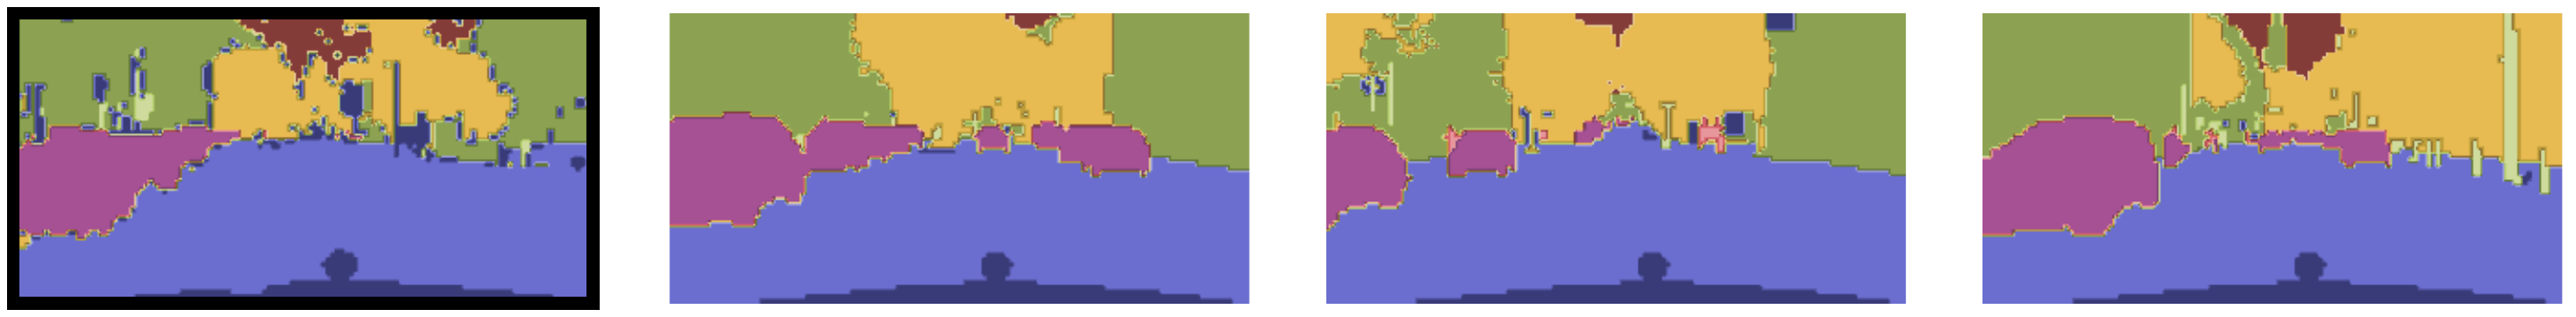}
	\end{subfigure}
	\caption{Analogous as in Figure \ref{fig:MNIST_similarity} but with the Cityscapes dataset . The leftmost column, marked with a black border, shows samples of our model. The remaining images are the closest one chosen from the training set.   }
 \label{fig:cityscapes_similarity}
\end{figure}
